# Supplementary material for: Optimal Algorithms for Mean Estimation under Local Differential Privacy
Source: arXiv:2205.02466 source file (2022-05-05)
Supplement: Supplementary file 1 [file appendix-opt-agg.tex]

\section{Optimality of \pu~with additive aggregation}
\label{sec:apdx-opt-agg}
In the previous section we have proved optimality of \pu~for a singe sample, assuming the output space of the randomizer is $\r^d$. In this section, we show that these assumptions are not necessary: we prove that \pu~with additive aggregation of outputs achieves the smallest variance among all estimators which are unbiased.

Given a randomizer $\R : \sphere^{d-1} \to \domain$ where $\domain$ is any general domain and an aggregation method $\A : \domain^n \to \R^d$, we define its error for $n$ samples
\begin{equation*}
    \err_n(\A,\R) = \sup_{v_1,\dots,v_n \in \sphere^{d-1}}\E \left[ \ltwo{\A(\R(v_1),\dots,\R(v_n)) -  \sum_{i=1}^n v_i}^2 \right].
\end{equation*}
The main result of this section is that the optimal choice of $\A$ and $\R$ is essentially additive aggregation with $\pu$. 
Let $\AdA$ denote additive aggregation, that is, $\AdA(u_1,\dots,u_n) = \sum_{i=1}^n u_i$.
The following theorem states our main result.
\begin{theorem}
\label{thm:opt-agg}
    Let $(\R,\A)$ be such that $\R$ is $\diffp$-DP local randomizer and $\E[\A(\R(v_1),\dots,\R(v_n))] = \sum_{i=1}^n v_i$ for all $v_1,\dots,v_n \in \sphere^{d-1}$. Then there is $p^\star \in [0,1]$ and $\gamma^\star \in [0,1]$ such that $\pu(p^\star,\gamma^\star)$ is $\diffp$-DP local randomizer and
    \begin{equation*}
        \err_n(\A,\R) \ge \err_n(\AdA,\pu(p^\star,\gamma^\star)).
    \end{equation*}
\end{theorem}

To prove~\Cref{thm:opt-agg}, we begin with the following lemma.
\begin{lemma}
\label{lemma:var-decomp}
    Let $P$ be a probability distribution over $\sphere^{d-1}$ such that $\E_{v \sim P}[v] = 0$.
    There is $\hat \R_i : \sphere^{d-1} \to \r^d$ for $i \in [n]$ such that $\hat \R_i$ is $\diffp$-DP local randomizer, $\E[\hat \R_i(v)] = v$ for all $v \in \sphere^{d-1}$, and
    \begin{equation*}
     \E_{v_1,\dots,v_n \sim P} \left[ \ltwo{\A(\R(v_1),\dots,\R(v_n)) -  \sum_{i=1}^n v_i}^2 \right]
        \ge \sum_{i=1}^n \E_{v_i \sim P} \left[ \ltwo{\hat \R_i(v_i) - v_i }^2 \right].  
    \end{equation*}
\end{lemma}

Before proving~\Cref{lemma:var-decomp}, we now complete the proof the~\Cref{thm:opt-agg}.
\begin{proof}(\Cref{thm:opt-agg})
    Let $P$ be the uniform distribution over the sphere $\sphere^{d-1}$. First, note that 
    \begin{align*}
     \err_n(\A,\R) 
        & = \sup_{v_1,\dots,v_n \in \sphere^{d-1}}\E \left[ \ltwo{\A(\R(v_1),\dots,\R(v_n)) -  \sum_{i=1}^n v_i}^2 \right] \\
        & \ge \E_{v_1,\dots,v_n \sim P} \left[ \ltwo{\A(\R(v_1),\dots,\R(v_n)) -  \sum_{i=1}^n v_i}^2 \right] \\
        &  \ge \sum_{i=1}^n \E_{v_i \sim P} \left[ \ltwo{\hat \R_i(v_i) - v_i }^2 \right].  
    \end{align*}
    Now we define $\R'_i$ similarly to the rotation-invariance lemma (\Cref{lemma:symmetry}). First, sample a random rotation matrix $U \in \r^{d \times d}$ where $U^T U = I$, then set
    \begin{equation*}
        \R'_i(v) = U^T \hat\R_i(Uv).
    \end{equation*}
    Note that for all $v \in \sphere^{d-1}$
    \begin{align*}
    \E[\ltwo{\R'_i(v) - v}^2] 
        & = \E_{U} [\ltwo{U^T\hat\R_i(Uv) - v}^2] \\
        & = \E_{U} [\ltwo{\hat\R_i(Uv) - U v}^2] \\
        & = \E_{v \sim P } [\ltwo{\hat\R_i(v) - v}^2].
    \end{align*}
    Overall, we have
    \begin{align*}
     \err_n(\A,\R) 
        &  \ge \sum_{i=1}^n \E_{v_i \sim P} \left[ \ltwo{\hat \R_i(v_i) - v_i }^2 \right] \\
        & = \sum_{i=1}^n \sup_{v \in \sphere^{d-1}} \E[\ltwo{\R'_i(v) - v}^2] \\
        & = \sum_{i=1}^n \err_1(\R'_i) \\
        & \stackrel{(i)}{\ge} \sum_{i=1}^n \err_1(\pu(p^\star,\gamma^\star)) \\
        & = \err_n(\AdA,\pu(p^\star,\gamma^\star)),
    \end{align*}
    where $(i)$ follows follows from our optimality result when $n=1$ (\Cref{thm:opt-repl}). The claim follows.
\end{proof}

Now we prove~\Cref{lemma:var-decomp}. 
\begin{proof}(\Cref{lemma:var-decomp})
    We define $\hat \R_i$ to be
    \begin{equation*}
        \hat \R_i(v_i) = \E_{v_j \sim P, j \neq i} [\A(\R(v_1),\dots,\R(v_n))] .
    \end{equation*}
    Note that $\hat \R_i$ is $\diffp$-DP local randomizer as it requires a single application of $\R(v_i)$. Moreover, $\E[\hat R_i(v)] = v$ for all $v \in \sphere^{d-1}$. We define 
    \begin{equation*}
        \hat \R_{\le i}(v_1,\dots,v_i) = \E_{v_j \sim P, j > i} \left[\A(\R(v_1),\dots,\R(v_n)) - \sum_{j=1}^i v_j \right],
    \end{equation*}
    and $\hat \R_0 = 0$.
    We now have
    \begin{align*}
     & \E_{v_1,\dots,v_n \sim P} \left[ \ltwo{\A(\R(v_1),\dots,\R(v_n)) -  \sum_{i=1}^n v_i}^2 \right]  \\
        & \quad = \E_{v_1,\dots,v_n \sim P} \left[ \ltwo{ \hat \R_{\le n}(v_1,\dots,v_n)   }^2 \right] \\
        &  \quad = \E_{v_1,\dots,v_n \sim P} \left[ \ltwo{ \hat \R_{\le n}(v_1,\dots,v_n) - \hat \R_{\le n-1}(v_1,\dots,v_{n-1}) + \hat \R_{\le n-1}(v_1,\dots,v_{n-1})    }^2 \right] \\
        & \quad  \stackrel{(i)}{=} \E_{v_1,\dots,v_n \sim P} \left[ \ltwo{ \hat \R_{\le n}(v_1,\dots,v_n) - \hat \R_{\le n-1}(v_1,\dots,v_{n-1}) }^2 \right] +  \E_{v_1,\dots,v_{n-1} \sim P} \left[ \ltwo{\hat \R_{\le n-1}(v_1,\dots,v_{n-1})    }^2 \right] \\
        & \quad  \stackrel{(ii)}{=} \sum_{i=1}^n \E_{v_1,\dots,v_i \sim P} \left[ \ltwo{ \hat \R_{\le i}(v_1,\dots,v_i) - \hat \R_{\le i-1}(v_1,\dots,v_{i-1}) }^2 \right] \\
        & \quad  \stackrel{(iii)}{\ge} \sum_{i=1}^n \E_{v_i \sim P} \left[ \ltwo{ E_{v_1,\dots,v_{i-1} \sim P} \left[ \hat \R_{\le i}(v_1,\dots,v_i) - \hat \R_{\le i-1}(v_1,\dots,v_{i-1})\right] }^2 \right] \\
        & \quad  \stackrel{(iv)}{=} \sum_{i=1}^n \E_{v_i \sim P} \left[ \ltwo{\hat \R_i(v_i) - v_i}^2 \right] \\
    \end{align*}
    where $(i)$ follows since $E_{v_n \sim P} [\R_{\le n}(v_1,\dots,v_n)] = \hat \R_{\le n-1}(v_1,\dots,v_{n-1})$, $(ii)$ follows by induction, $(iii)$ follows from Jensen's inequality, and $(iv)$ follows since $E_{v_1,\dots,v_{i-1} \sim P} [ \hat \R_{\le i}(v_1,\dots,v_i)] = \hat \R_i(v_i) - v_i$ and $E_{v_1,\dots,v_{i-1} \sim P} [ \hat \R_{\le i-1}(v_1,\dots,v_{i-1})] = 0$.

\end{proof}
